# Supplementary material for: Scalable Surface Reconstruction with Delaunay-Graph Neural Networks
Source: arXiv:2107.06130 source file (2022-02-02)
Supplement: Supplementary file 2 [file supp_uncleaned.tex]

% Please add the following required packages to your document preamble:
% \usepackage{multirow}
% \usepackage{graphicx}
% \usepackage[table,xcdraw]{xcolor}
% If you use beamer only pass "xcolor=table" option, i.e. \documentclass[xcolor=table]{beamer}
\begin{table*}[]
\resizebox{\textwidth}{!}{%
\begin{tabular}{
>{\columncolor[HTML]{FFFFFF}}l |
>{\columncolor[HTML]{FFFFFF}}c 
>{\columncolor[HTML]{FFFFFF}}c 
>{\columncolor[HTML]{FFFFFF}}c |
>{\columncolor[HTML]{FFFFFF}}c 
>{\columncolor[HTML]{FFFFFF}}c 
>{\columncolor[HTML]{FFFFFF}}c |
>{\columncolor[HTML]{FFFFFF}}c 
>{\columncolor[HTML]{FFFFFF}}c 
>{\columncolor[HTML]{FFFFFF}}c }
\hline
 & \multicolumn{3}{c|}{\cellcolor[HTML]{FFFFFF}} & \multicolumn{3}{c|}{\cellcolor[HTML]{FFFFFF}} & \multicolumn{3}{c}{\cellcolor[HTML]{FFFFFF}} \\
 & \multicolumn{3}{c|}{\multirow{-2}{*}{\cellcolor[HTML]{FFFFFF}Vu \textit{et al.} \cite{Vu2012}}} & \multicolumn{3}{c|}{\multirow{-2}{*}{\cellcolor[HTML]{FFFFFF}Jancosek \textit{et al.} \cite{Jancosek2014}}} & \multicolumn{3}{c}{\multirow{-2}{*}{\cellcolor[HTML]{FFFFFF}Ours}} \\
scene & \multicolumn{1}{l}{\cellcolor[HTML]{FFFFFF}Completen.} & \multicolumn{1}{l}{\cellcolor[HTML]{FFFFFF}Accuracy} & \multicolumn{1}{l|}{\cellcolor[HTML]{FFFFFF}F1-score} & \multicolumn{1}{l}{\cellcolor[HTML]{FFFFFF}Completen.} & \multicolumn{1}{l}{\cellcolor[HTML]{FFFFFF}Accuracy} & \multicolumn{1}{l|}{\cellcolor[HTML]{FFFFFF}F1-score} & \multicolumn{1}{l}{\cellcolor[HTML]{FFFFFF}Completen.} & \multicolumn{1}{l}{\cellcolor[HTML]{FFFFFF}Accuracy} & \multicolumn{1}{l}{\cellcolor[HTML]{FFFFFF}F1-score} \\ \hline
kicker & \textbf{0.82} & \textbf{0.77} & \textbf{0.79} & 0.82 & 0.69 & 0.75 & 0.79 & 0.73 & 0.76 \\
pipes & 0.78 & 0.80 & \textbf{0.79} & \textbf{0.78} & 0.76 & 0.77 & 0.67 & \textbf{0.88} & 0.76 \\
delivery\_area & \textbf{0.88} & 0.58 & 0.70 & 0.87 & 0.53 & 0.66 & 0.80 & \textbf{0.64} & \textbf{0.71} \\
meadow & 0.76 & 0.39 & 0.52 & \textbf{0.78} & 0.37 & 0.51 & 0.68 & \textbf{0.51} & \textbf{0.58} \\
office & 0.62 & 0.69 & \textbf{0.65} & \textbf{0.62} & 0.56 & 0.59 & 0.47 & \textbf{0.81} & 0.59 \\
playground & \textbf{0.77} & 0.63 & 0.70 & 0.76 & 0.54 & 0.63 & 0.76 & \textbf{0.65} & \textbf{0.70} \\
terrains & 0.81 & \textbf{0.74} & \textbf{0.78} & 0.81 & 0.71 & 0.76 & \textbf{0.83} & 0.69 & 0.75 \\
terrace & \textbf{0.86} & 0.68 & 0.76 & 0.86 & 0.66 & 0.74 & 0.83 & \textbf{0.83} & \textbf{0.83} \\
relief & \textbf{0.83} & 0.56 & 0.67 & 0.82 & 0.53 & 0.64 & 0.75 & \textbf{0.86} & \textbf{0.80} \\
relief\_2 & \textbf{0.82} & 0.58 & 0.68 & 0.82 & 0.56 & 0.67 & 0.73 & \textbf{0.85} & \textbf{0.79} \\
electro & \textbf{0.84} & 0.51 & 0.64 & 0.84 & 0.47 & 0.60 & 0.83 & \textbf{0.58} & \textbf{0.68} \\
courtyard & 0.85 & 0.67 & 0.75 & 0.85 & 0.62 & 0.72 & \textbf{0.86} & \textbf{0.69} & \textbf{0.77} \\
facade & 0.66 & 0.43 & 0.52 & \textbf{0.66} & 0.41 & 0.50 & 0.50 & \textbf{0.56} & \textbf{0.53} \\ \hline
mean & \textbf{0.793} & 0.619 & 0.688 & 0.793 & 0.569 & 0.657 & 0.731 & \textbf{0.714} & \textbf{0.712} \\ \hline
\end{tabular}%
}
\caption{Results of all scenes of the train dataset of ETH3D \cite{Schops2017} for uncleaned mesh reconstructions at distance $\tau = 5 cm$. The best (highest) values for Completeness (Completen.), Accuracy and F1-score per scene are in bold letters.}
\label{tab:supp_uncleaned}
\end{table*}
